# Supplementary material for: GaussianMamba: Geometric and Relational State Space Scanning of 3D Gaussian Primitives
Source: arXiv:2611.22742 source file (2026-11-17)
Supplement: Supplementary file 1 [file X_suppl.tex]

\clearpage
\setcounter{page}{1}
\maketitlesupplementary

\subsection{Evaluation Protocol and Metric Definitions}
We analyze the spatial, geometric, and semantic properties of Gaussian ordering strategies. Each ordering defines a permutation $\pi$ of $N$ Gaussian primitives, where $\pi_t$ denotes the Gaussian at sequence position $t$.

To characterize Gaussian geometry, we construct a compact shape descriptor from the decoded positive scales:
\begin{equation}
\mathbf{g}_i =
\left[
\frac{s_i^{\min}}{s_i^{\max}},
\frac{s_i^{\mathrm{mid}}}{s_i^{\max}},
\log(s_i^{\min}s_i^{\mathrm{mid}}s_i^{\max})
\right].
\label{eq:supp_shape_descriptor}
\end{equation}
Here, $s_i^{\min}$, $s_i^{\mathrm{mid}}$, and $s_i^{\max}$ denote the sorted Gaussian scales. For distance evaluation, each descriptor dimension is standardized within its sample, yielding $\hat{\mathbf{g}}_i$.

We measure spatial and geometric continuity between consecutive sequence elements as
\begin{equation}
\begin{aligned}
d_t^{\mathrm{spa}}
&= \|\boldsymbol{\mu}_{\pi_t}
-\boldsymbol{\mu}_{\pi_{t+1}}\|_2,\\
d_t^{\mathrm{shape}}
&= \|\hat{\mathbf{g}}_{\pi_t}
-\hat{\mathbf{g}}_{\pi_{t+1}}\|_2,
\end{aligned}
\label{eq:supp_step_metrics}
\end{equation}
where $\boldsymbol{\mu}_i$ is the Gaussian center in world coordinates. Mean spatial and shape steps are obtained by averaging these distances over consecutive sequence pairs.

Semantic adjacency measures the proportion of valid consecutive Gaussian pairs that share the same predicted semantic label:
\begin{equation}
A_{\mathrm{sem}} =
\frac{1}{|\mathcal{V}|}
\sum_{t\in\mathcal{V}}
\mathbb{I}
\left[
\hat{y}_{\pi_t}
=\hat{y}_{\pi_{t+1}}
\right],
\label{eq:supp_semantic_adjacency}
\end{equation}
where $\mathcal{V}$ contains consecutive pairs with valid predicted labels. Local semantic purity extends this evaluation to sequence offsets of up to eight positions.

Finally, we quantify ordering complementarity using the mean Jaccard overlap of sequence neighborhoods:
\begin{equation}
O(a,b)=\frac{1}{N}\sum_{i=1}^{N}
\frac{
|\mathcal{N}_i^{a}\cap\mathcal{N}_i^{b}|
}{
|\mathcal{N}_i^{a}\cup\mathcal{N}_i^{b}|
},
\label{eq:supp_neighbor_overlap}
\end{equation}
where $\mathcal{N}_i^{a}$ and $\mathcal{N}_i^{b}$ contain up to eight preceding and eight following Gaussian neighbors under orderings $a$ and $b$. Lower overlap indicates more distinct sequence neighborhoods, rather than necessarily better prediction performance.


\subsection{Sensitivity to Vertical Ordering Range}
Table~\ref{tab:supp_z_range} investigates the influence of vertical quantization bounds on center-based and support-aware Morton ordering. Unlike conventional Morton ordering, the support-aware variant replaces the Gaussian
center's vertical coordinate with its upper support position:
\begin{equation}
z_i^{\mathrm{sup}} = \mu_{i,z} + \sqrt{[\boldsymbol{\Sigma}_i]_{zz}},
\label{eq:supp_vertical_support}
\end{equation}
where $\boldsymbol{\Sigma}_i$ denotes the Gaussian covariance matrix.

The analysis reveals that 14.27\% of upper support positions exceed the original 3 m boundary, reaching approximately 3.64 m. Consequently, we adopt an upper ordering bound of 4 m to represent the observed vertical support without clipping.

Although larger bounds can reduce spatial transition distances, they do not consistently improve geometric continuity. Moreover, support-aware Morton achieves only modest locality differences compared with center-based Morton under matched ranges. Our selection therefore prioritizes support coverage rather than claiming superior spatial locality. The Gaussian representation range remains unchanged.

\begin{table}[t]
\centering
\caption{Effect of the vertical range on Morton ordering.}
\label{tab:supp_z_range}
\small
\setlength{\tabcolsep}{4pt}
\resizebox{\columnwidth}{!}{%
\begin{tabular}{@{}ccccc@{}}
\toprule
\textbf{$z_{\max}$}
& \textbf{Center Step $\downarrow$}
& \textbf{Support Step $\downarrow$}
& \textbf{Center CrossGeo $\downarrow$}
& \textbf{Support CrossGeo $\downarrow$} \\
\midrule
3 & 3.185 & 3.090 & 0.476 & 0.457 \\
\textbf{4} & 3.149 & 3.148 & 0.480 & 0.458 \\
5 & 3.033 & 3.037 & 0.485 & 0.463 \\
6 & 2.947 & 2.997 & 0.489 & 0.466 \\
8 & 2.809 & 2.858 & 0.509 & 0.480 \\
\bottomrule
\end{tabular}%
}
\end{table}



\subsection{Complementarity of Gaussian Ordering Strategies}
We examine whether spatial, semantic, and geometric ordering strategies generate distinct sequence neighborhoods using the overlap metric in Eq.~\ref{eq:supp_neighbor_overlap}.

As reported in Table~\ref{tab:supp_complementarity}, Semantic-Support and Local-Geo-Support exhibit a neighborhood overlap of 0.327, indicating that the two strategies expose substantially different local relationships. Their overlap with conventional support-based Morton ordering is also limited, suggesting that semantic and geometric reordering introduce neighborhoods beyond those defined by spatial proximity alone.

Importantly, both strategies retain the spatial organization established by Morton while rearranging primitives within local regions. These observations motivate our two complementary scanning branches, which capture different relationships without requiring independent global spatial partitioning.

Nevertheless, neighborhood diversity alone does not establish an occupancy performance improvement. Its effectiveness is evaluated through the scanning ablations
in Table~\ref{tab:scanning_ablation}.

The support-based overlap measurements in Table~\ref{tab:supp_complementarity} use the diagnostic $z_{\max}=3$ configuration.
\begin{table}[t]
\centering
\caption{Neighbor overlap between Gaussian ordering strategies.}
\label{tab:supp_complementarity}
\small
\setlength{\tabcolsep}{4pt}
\begin{tabular}{@{}lc@{}}
\toprule
\textbf{Ordering Pair} & \textbf{Overlap} \\
\midrule
Center-Morton / Semantic-Center & 0.302 \\
Center-Morton / Local-Geo-Center & 0.193 \\
Semantic-Center / Local-Geo-Center & 0.328 \\
\midrule
Support-Morton / Semantic-Support & 0.177 \\
Support-Morton / Local-Geo-Support & 0.129 \\
Semantic-Support / Local-Geo-Support & 0.327 \\
\bottomrule
\end{tabular}
\end{table}


\subsection{Class-wise Semantic Locality}
Table~\ref{tab:supp_class_locality} examines the semantic locality induced by conventional spatial ordering across
different Gaussian categories.

For each class, locality is measured as the ratio of consecutive same-class pairs to valid consecutive pairs containing at least one Gaussian from that class.
This evaluates class-specific sequence organization rather than classification accuracy.

Hilbert consistently improves locality over lexicographic XYZ ordering across the evaluated categories. For instance, locality increases from 0.1301 to 0.3528
for cars and from 0.2748 to 0.6366 for driveable surfaces.

However, locality varies considerably between compact object categories and large structural regions. These findings demonstrate that spatial ordering can implicitly capture semantic relationships, but it does not explicitly optimize them. Our semantic-structural ordering therefore builds upon spatial organization while
introducing class-aware relationships within local Gaussian neighborhoods.

\begin{table}[ht]
\centering
\caption{Class-wise semantic locality under spatial ordering.}
\label{tab:supp_class_locality}
\small
\setlength{\tabcolsep}{3pt}
\resizebox{\columnwidth}{!}{%
\begin{tabular}{@{}lrrrrr@{}}
\toprule
\textbf{Class}
& \textbf{\#Gauss}
& \textbf{Random}
& \textbf{XYZ}
& \textbf{Hilbert}
& \textbf{Gain} \\
\midrule
Bicycle     & 1,583     & 0.0003 & 0.0374 & 0.0681 & 0.0307 \\
Bus         & 63,795    & 0.0071 & 0.1519 & 0.3288 & 0.1769 \\
Car         & 359,471   & 0.0217 & 0.1301 & 0.3528 & 0.2227 \\
Motorcycle  & 9,475     & 0.0008 & 0.0307 & 0.0904 & 0.0596 \\
Pedestrian  & 29,197    & 0.0018 & 0.0338 & 0.1311 & 0.0973 \\
Truck       & 89,609    & 0.0077 & 0.1302 & 0.2657 & 0.1356 \\
Driveable   & 1,387,573 & 0.0649 & 0.2748 & 0.6366 & 0.3618 \\
Vegetation  & 3,204,108 & 0.2004 & 0.3784 & 0.6993 & 0.3210 \\
\bottomrule
\end{tabular}%
}
\end{table}



\subsection{Ordering Behavior Across Prediction Quality}
To investigate whether the observed ordering properties depend on occupancy prediction quality, we divide the samples into low-, medium-, and high-mIoU groups using the lower and upper quartiles.

As presented in Table~\ref{tab:supp_quality}, semantic adjacency remains approximately 0.934 across all groups, despite substantial differences in occupancy mIoU. Similarly, semantic--geometric neighborhood overlap
varies only slightly, remaining close to 0.327.

These observations indicate that the measured sequence relationships are not restricted to samples with high occupancy prediction accuracy. Furthermore, the
results suggest that improved occupancy performance does not necessarily lead to stronger ordering locality.

Nevertheless, occupancy mIoU does not directly quantify how accurately individual Gaussian primitives fit object geometry. We therefore interpret this experiment as a robustness analysis of sequence organization rather than
a measure of Gaussian fitting quality.

\begin{table}[ht]
\centering
\caption{Ordering properties across prediction quality groups.}
\label{tab:supp_quality}
\small
\setlength{\tabcolsep}{4pt}
\resizebox{\columnwidth}{!}{%
\begin{tabular}{@{}lccccc@{}}
\toprule
\textbf{Quality}
& \textbf{N}
& \textbf{mIoU (\%)}
& \textbf{Sem. Adj.}
& \textbf{Geo. Shape}
& \textbf{Overlap} \\
\midrule
Low    & 125 & 26.89 & 0.9339 & 0.1158 & 0.3275 \\
Medium & 250 & 37.99 & 0.9334 & 0.1175 & 0.3269 \\
High   & 125 & 51.00 & 0.9355 & 0.1263 & 0.3266 \\
\bottomrule
\end{tabular}%
}
\end{table}


\subsection{Spatial and Geometric Transitions}
We further analyze the distribution of spatial and geometric transitions to characterize the limitations
of purely position-based ordering.

As shown in Table~\ref{tab:supp_transitions}, Hilbert produces the most spatially continuous sequences, with only 9.13\% of consecutive transitions exceeding 5 m. In contrast, Semantic-Support and Local-Geo-Support exhibit higher long-distance transition rates of 37.67\% and 52.11\%, respectively.

However, these strategies substantially reduce geometric dissimilarity. The 90th-percentile shape transition
decreases from 0.795 under Hilbert ordering to 0.344 for Semantic-Support and 0.212 for Local-Geo-Support.

These results demonstrate that spatial continuity and geometric similarity represent different objectives in Gaussian sequence construction. This trade-off motivates our spatially constrained ordering design, where Support-Aware Morton provides the spatial foundation, while semantic and geometric properties determine the local scanning order.
\begin{table}[ht]
\centering
\caption{Spatial jump rates and geometric transition tails.}
\label{tab:supp_transitions}
\small
\setlength{\tabcolsep}{4pt}
\resizebox{\columnwidth}{!}{%
\begin{tabular}{@{}lcccc@{}}
\toprule
\textbf{Ordering}
& \textbf{Jump $>$5m $\downarrow$}
& \textbf{Jump $>$10m $\downarrow$}
& \textbf{Spatial P90 $\downarrow$}
& \textbf{Shape P90 $\downarrow$} \\
\midrule
Random
& 0.9943 & 0.9717 & 82.265 & 4.044 \\
XYZ
& 0.3966 & 0.1125 & 10.690 & 2.575 \\
Hilbert
& \textbf{0.0913} & \textbf{0.0041} & \textbf{4.881} & 0.795 \\
Morton
& 0.1396 & 0.0255 & 5.544 & 0.869 \\
Support-Morton
& 0.1355 & 0.0254 & 5.498 & 0.864 \\
\midrule
Semantic-Support
& 0.3767 & 0.0993 & 9.971 & 0.344 \\
Local-Geo-Support
& 0.5211 & 0.1641 & 11.871 & \textbf{0.212} \\
\bottomrule
\end{tabular}%
}
\end{table}



\textbf{Analysis of Gaussian Ordering Strategies.} Table~\ref{tab:gaussian_ordering_analysis}
compares the spatial, geometric, and semantic
 roperties of different Gaussian ordering strategies. Spatial and shape steps measure consecutive Gaussian distances in 3D space and standardized scale-descriptor space. Semantic adjacency and purity evaluate predicted-label consistency along the resulting sequences. Detailed metric definitions are provided in the supplementary material.



Conventional spatial orderings substantially improve
locality over random sequencing, with Hilbert achieving
the shortest spatial transitions (2.828 m). However, spatial proximity alone does not explicitly account for the geometric and semantic attributes of Gaussian primitives. Semantic-Support increases predicted-label adjacency from 0.810 to 0.934 compared with Hilbert, while Local-Geo-Support reduces shape dissimilarity from 0.319 to 0.119. These improvements are accompanied by longer
spatial transitions, highlighting the trade-off between spatial continuity and Gaussian-specific structural relationships.

Motivated by these observations, we adopt a shared Support-Aware Morton scaffold to maintain spatial organization and introduce separate local semantic and geometric ordering strategies. This design constructs complementary scanning
sequences without discarding their common spatial foundation.


\textbf{Gaussian Scanning Ablation.} To examine whether the complementary ordering properties identified in
Table~\ref{tab:gaussian_ordering_analysis} translate into occupancy improvements, we evaluate spatial-only, semantic-aware, and geometry-aware Mamba scanning under a consistent training protocol.


\begin{table*}[t]
\centering
\caption{Spatial, geometric, and semantic locality of Gaussian ordering strategies.}
\label{tab:gaussian_ordering_analysis}
\small
\setlength{\tabcolsep}{9pt}
\begin{tabular}{@{}lcccc@{}}
\toprule
\textbf{Ordering}
& \textbf{Spatial Step (m) $\downarrow$}
& \textbf{Shape Step $\downarrow$}
& \textbf{Semantic Adj. $\uparrow$}
& \textbf{Semantic Purity $\uparrow$} \\
\midrule
Random                 & 49.652 & 1.216 & 0.362 & 0.362 \\
XYZ                    & 8.383  & 0.852 & 0.589 & 0.519 \\
Hilbert                & \textbf{2.828} & 0.319 & 0.810 & 0.754 \\
Morton                 & 3.185  & 0.346 & 0.801 & 0.744 \\
Support-Aware Morton   & 3.148  & 0.340 & 0.802 & 0.744 \\
\midrule
Semantic-Support       & 5.179  & 0.177 & \textbf{0.934} & \textbf{0.789} \\
Local-Geo-Support      & 6.560  & \textbf{0.119} & 0.743 & 0.720 \\
\bottomrule
\end{tabular}
\end{table*}
